# Supplementary material for: metabeta -- A fast neural model for Bayesian mixed-effects regression
Source: arXiv:2510.07473 source file (2026-02-04)

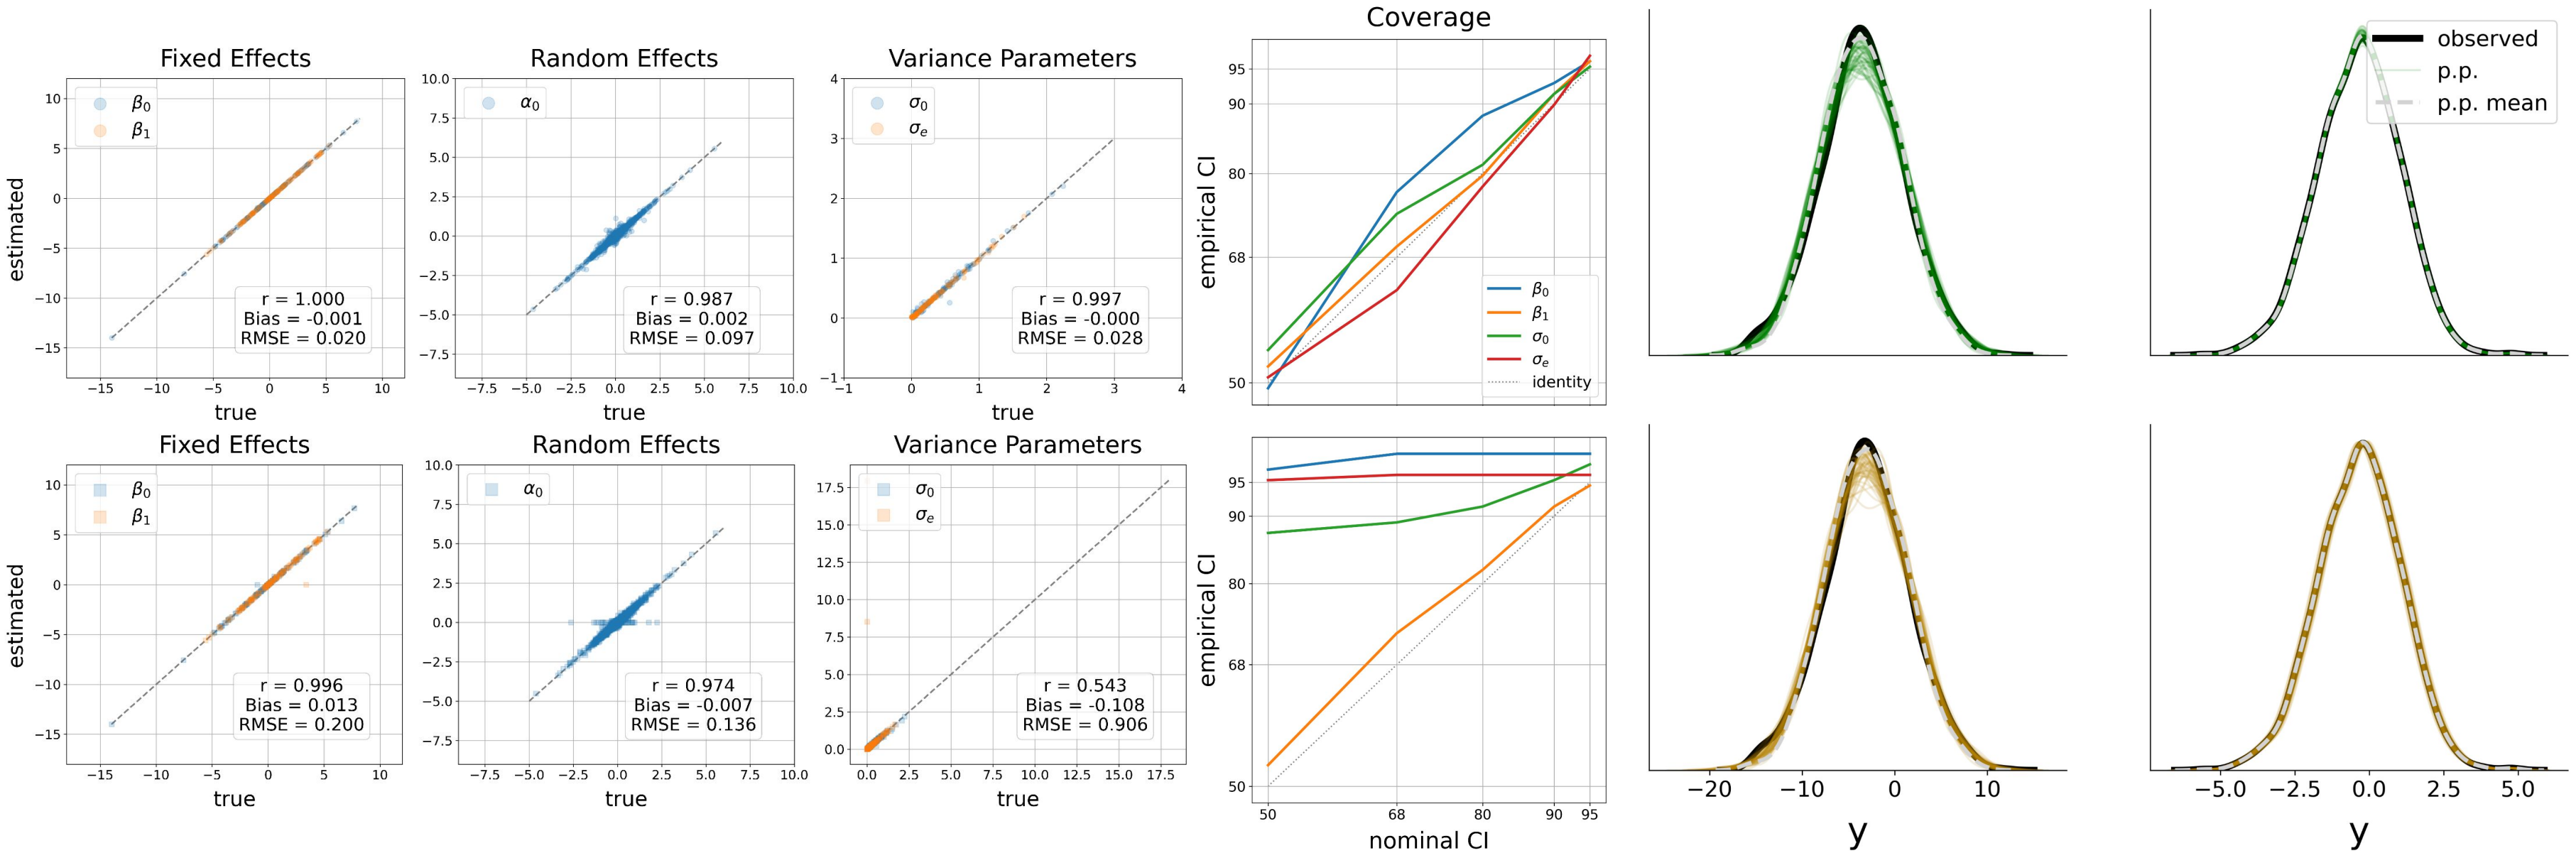

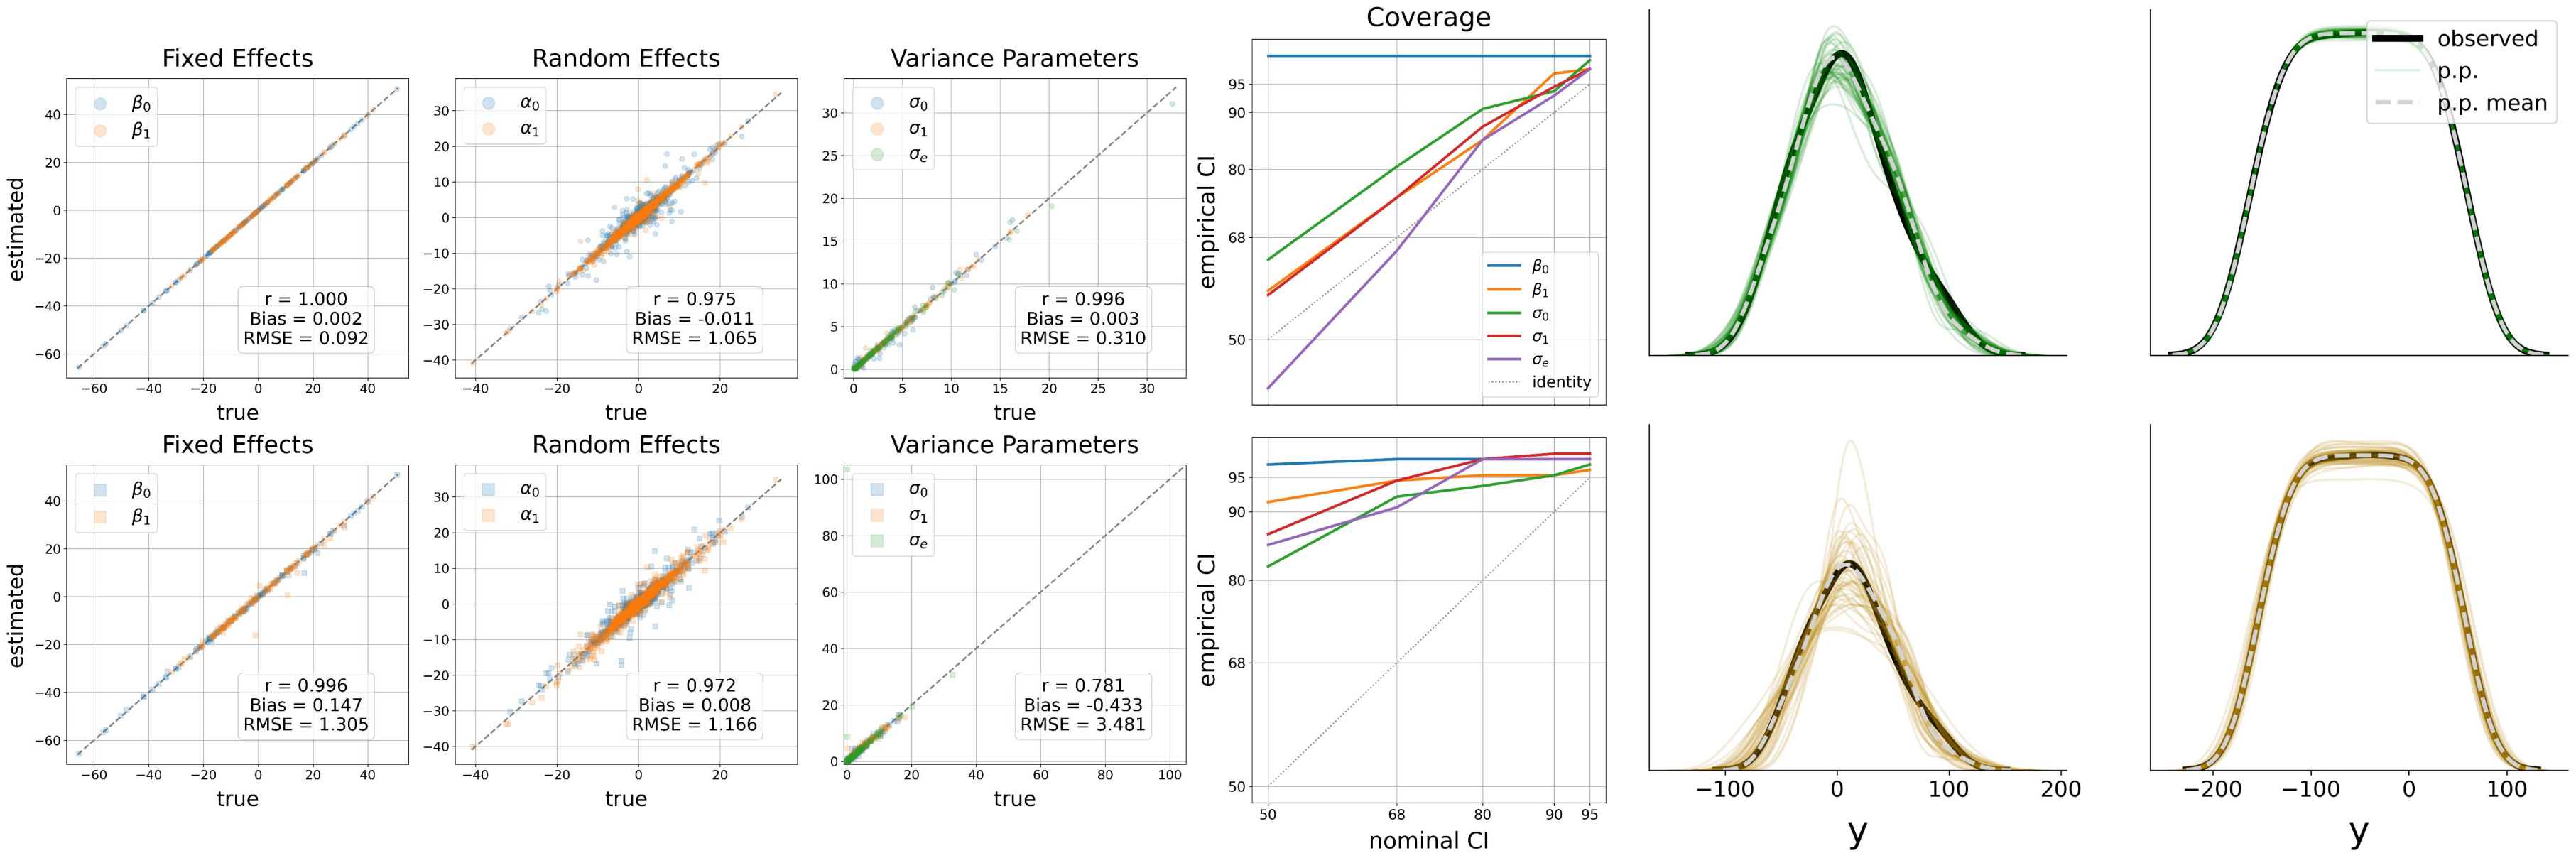

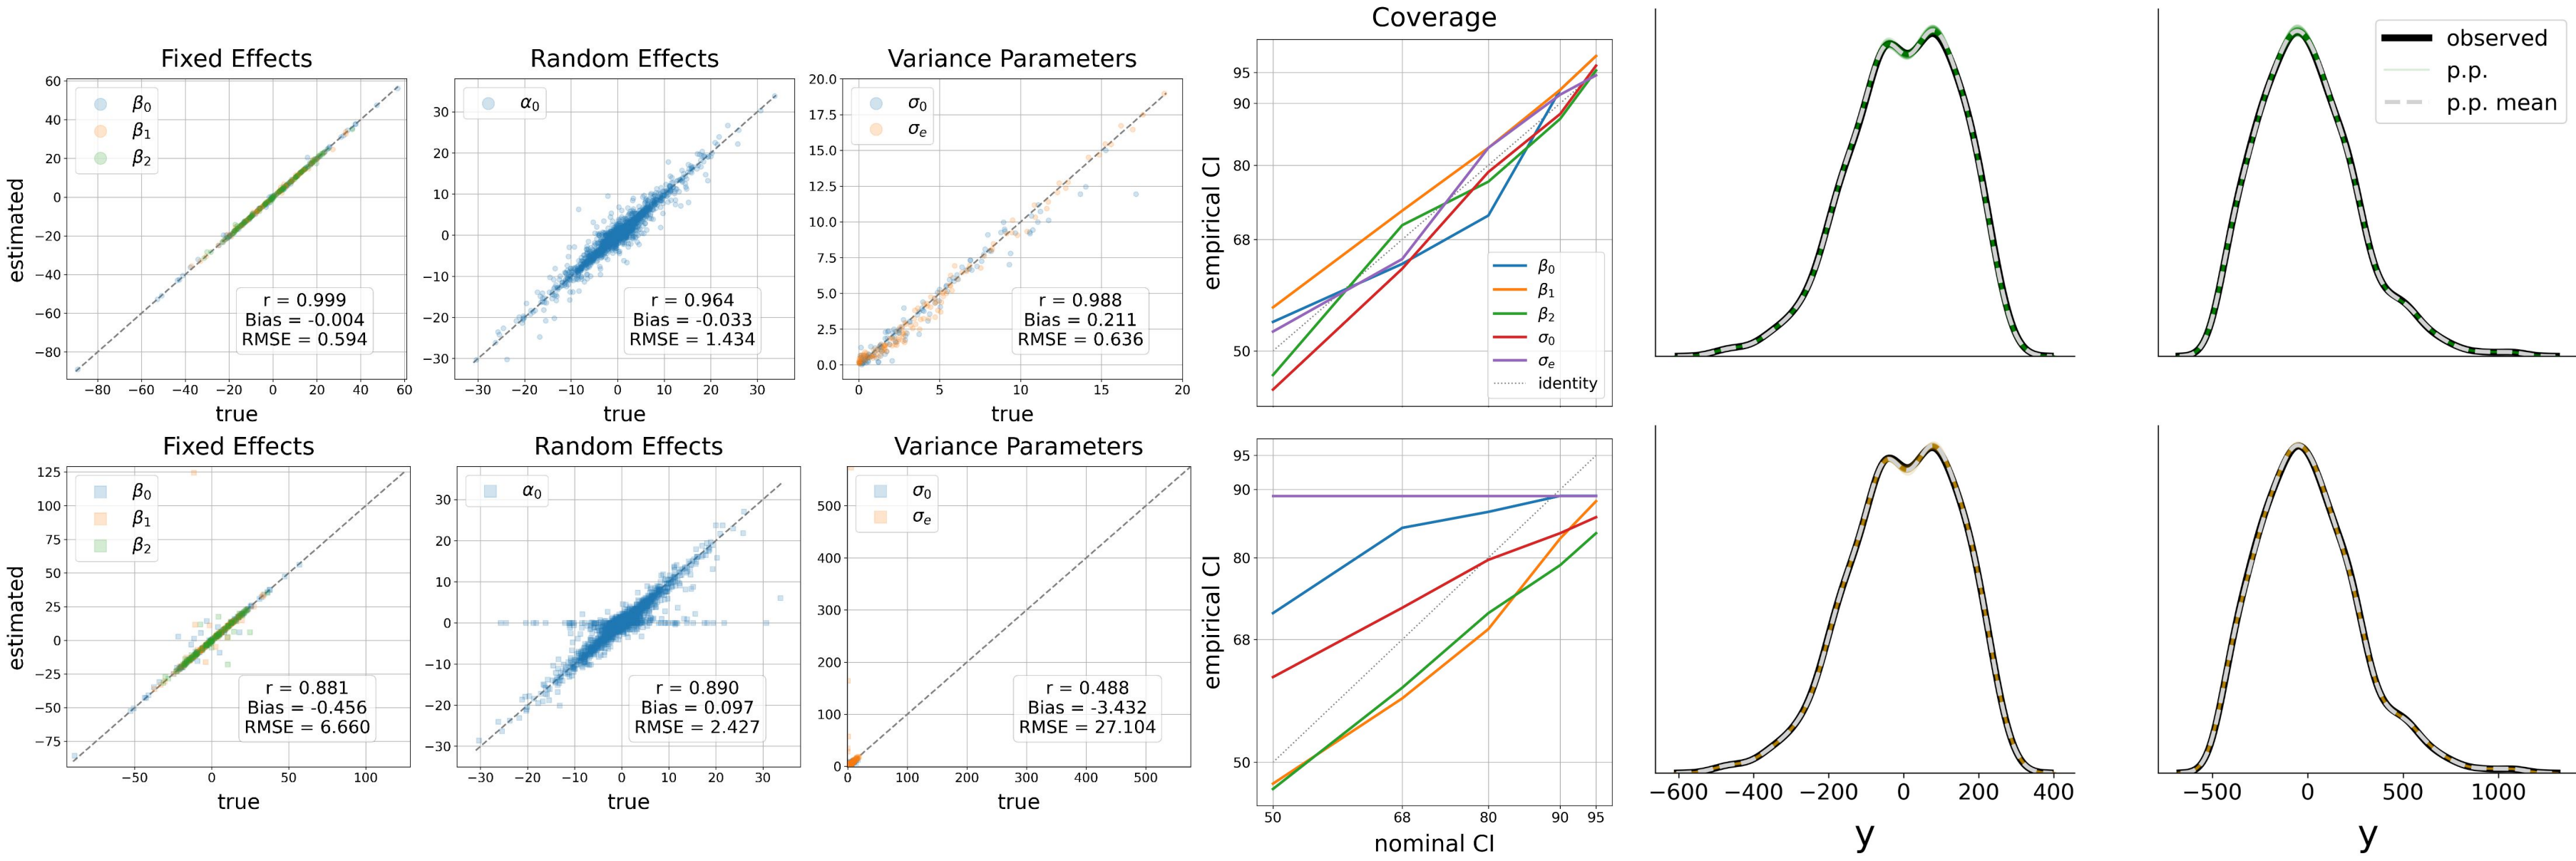



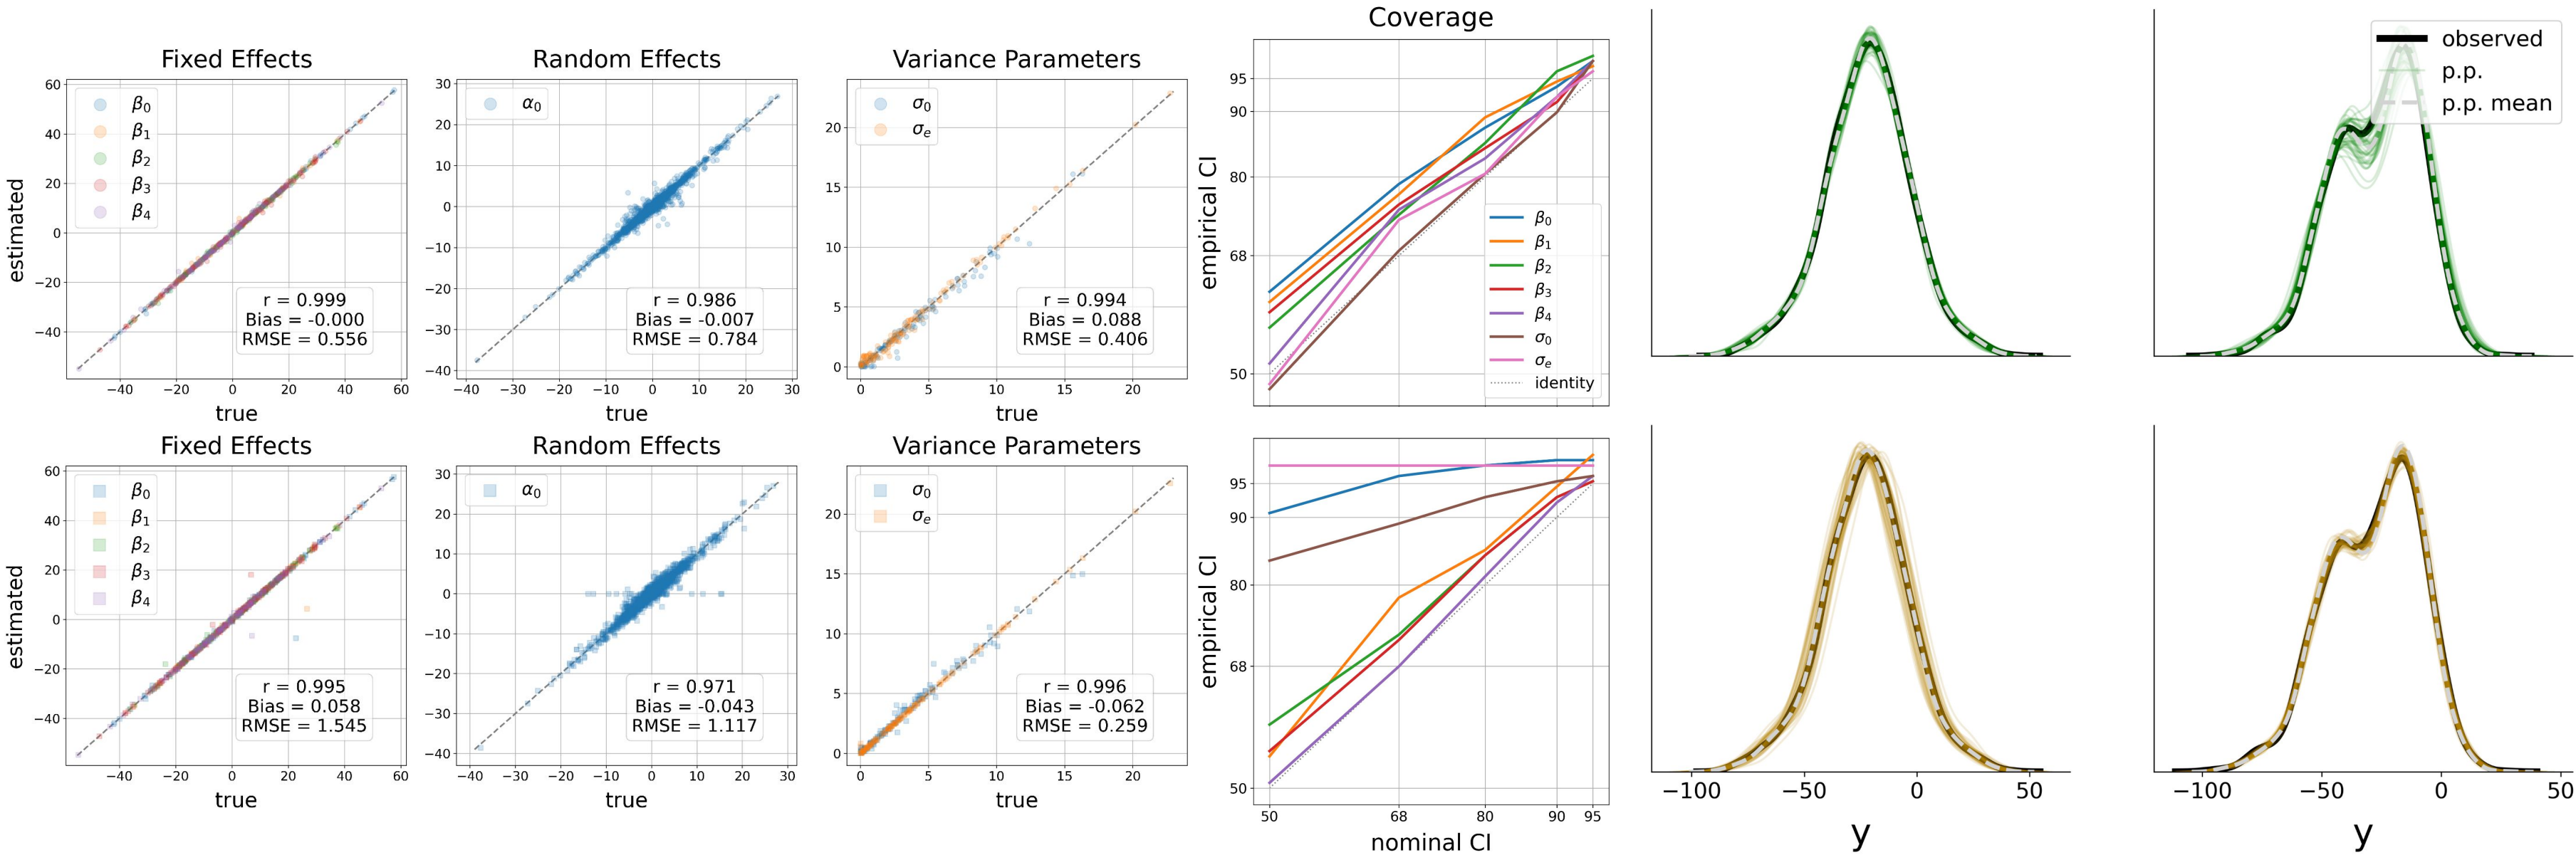

Supplement: Supplementary file 1 [file si_res.pdf]
